# Supplementary material for: Disentangling data distribution for Federated Learning
Source: arXiv:2410.12530 source file (2024-12-30)
Supplement: Supplementary file 1 [file AppendixC.tex]

\section{Formulation of FedAdOb in HFL and VFL}
Consider a neural network $f_\Theta(x):\calX \to \RR$, where $x \in \calX$, $\Theta$ denotes model parameters of neural networks. 

\noindent\textbf{VFL.} $K$ passive parties and one active party collaboratively optimize $\Theta = (\omega, \theta_1, \cdots, \theta_K)$ of network according to Eq. \eqref{eq:loss-VFL-app}.
\begin{equation}\label{eq:loss-VFL-app}
\begin{split}
        \min_{\omega, \theta_1, \cdots, \theta_K} &\frac{1}{n}\sum_{i=1}^n\ell(F_{\omega} \circ (G_{\theta_1}(x_{1,i}),G_{\theta_2}(x_{2,i}), \\
        & \cdots,G_{\theta_K}(x_{K,i})), y_{i}),
\end{split}
\end{equation}
where $\ell$ is the loss, e.g., the cross-entropy loss, passive party $P_k$ owns features $\calD_k = (x_{k,1}, \cdots, x_{k,n}) \in \mathcal{X}_k$ and the passive model $G_{\theta_k}$, the active party owns the labels $y \in \mathcal{Y}$ and active model $F_\omega$, $\mathcal{X}_k$ and $\mathcal{Y}$ are the feature space of party $P_k$ and the label space respectively. Furthermore, FedAdOb aims to optimize:
\begin{equation} \label{eq:loss-aof-vfl-app}
\begin{split}
        \min_{\omega, \theta_1,\cdots, \theta_K} &\frac{1}{N}\sum_{i=1}^N\ell(F_{\omega}g_{\omega} \circ (G_{\theta_1}(g_{\theta_1}(x_{1,i}, s_{p_1})), \\
        &\cdots, G_{\theta_K}(g_{\theta_K}(x_{K,i},s_{p_K})), y_{i}).
\end{split}
\end{equation}
Denote the composite function  $G_{\theta_j}g_{\theta_j}()$ as $G'_{\theta_j}()$, $j=1, \cdots, K$. Then we rewrite the Eq. \eqref{eq:loss-aof-vfl-app} as follows 
\begin{equation} 
\begin{split}
        \min_{\omega, \theta_1,\cdots, \theta_K} &\frac{1}{N}\sum_{i=1}^N\ell(F'_{\omega} \circ (G'_{\theta_1}(x_{1,i}, s^{p_1})), \\
        &\cdots, G'_{\theta_K}(x_{K,i}, s^{p_K})) , s^a, y_{i}),
\end{split}
\end{equation}

\noindent\textbf{HFL.} $K$  party collaboratively optimize $\Theta = (\omega, \theta_1, \cdots, \theta_K)$ of network according to Eq. \eqref{eq:loss-HFL-app}.
\begin{equation} \label{eq:loss-HFL-app}
    \min_{\theta_1, \cdots, \theta_K,\omega} \sum_{k=1}^K\sum_{i=1}^{n_k}\frac{\ell(F_\omega(x_{k,i}), y_{k,i})}{n_1+\cdots+n_K},
\end{equation}
where $\ell$ is the loss, e.g., the cross-entropy loss, $\calD_k=\{(x_{k,i}, y_{k,i})\}_{i=1}^{n_k}$ is the dataset with size $n_k$ owned by client $k$.
Furthermore, FedAdOb aims to optimize:
\begin{equation} \label{eq:loss-aof-app}
\begin{split}
        \min_{\omega, \theta_1,\cdots, \theta_K} &\frac{1}{N}\sum_{i=1}^N\ell(F_{\omega}g_{\omega} \circ (G_{\theta_1}(g_{\theta_1}(x_{1,i}, s_{p_1})), \\
        &\cdots, G_{\theta_K}(g_{\theta_K}(x_{K,i},s_{p_K})), y_{i}).
\end{split}
\end{equation}
Denote the composite function  $G_{\theta_j}g_{\theta_j}()$ as $G'_{\theta_j}()$, $j=1, \cdots, K$. Then we rewrite the Eq. \eqref{eq:loss-aof-app} as follows 
\begin{equation} \label{eq:loss-aof-HFL-app}
    \min_{\theta_1, \cdots, \theta_K,\omega} \sum_{k=1}^K\sum_{i=1}^{n_k}\frac{\ell(F_\omega \circ (G'_{\theta_k}(x_{k,i}, s_{p_k}), y_{k,i})}{n_1+\cdots+n_K},
\end{equation}

Then Proposition 1 ends the proof.
